# Supplementary material for: Quantifying Impairment and Disease Severity Using AI Models Trained on Healthy Subjects
Source: arXiv:2311.12781 source file (2023-11-21)
Supplement: Supplementary file 1 [file Appendix.tex]

\subsechttps://www.overleaf.com/project/641136b301f6b3ec0c4e17bd#tion{Distance-based Quantification Approach(appendix)} 
Comparing Healthy and Impaired Populations using FID Distance
The Fréchet Inception Distance (FID) (cite) is a commonly used metric to evaluate the similarity between two sets of feature representations extracted by a deep neural network. It is usually used for the task of image generation (cite) where FID distance helps to understand if the generated images are close to real images or not by comparing the feature representations of the generated and real images.

In our context of quantifying impairment, the FID distance can be used to compare the features of a healthy subject population with those extracted from an impaired subject, such as patients with a particular disease or condition. The idea is to assess whether the features of the impaired subject are significantly different from those of the healthy population, and if so, to what extent.

Let $x_1, x_2, ..., x_n$ be the feature representations of the healthy population, and $y_1, y_2, ..., y_m$ be the feature representations of the impaired subject. The mean and covariance matrices of these features are denoted by $\mu_x, \mu_y$ and $\Sigma_x, \Sigma_y$, respectively. The FID distance between the healthy population and the impaired subject is then calculated using the following formula:

$$ FID(x, y) = \|\mu_x - \mu_y\|_2^2 + Tr(\Sigma_x + \Sigma_y - 2(\Sigma_x \Sigma_y)^{1/2}) $$

where $Tr(\cdot)$ denotes the trace operator and $\|\cdot\|_2$ denotes the $L_2$ norm. A lower FID distance indicates a higher similarity between the two sets of features, while a higher FID distance indicates a greater difference.

To apply the FID distance to our problem, we, first, extract the feature representations of the images/sensor data from the two populations using a pre-trained deep neural network. The pre-trained network is trained to identify the low-level semantic labels that are indicative of the impairment. For example, in the case of stroke quantification, the network is trained to predict the primitives performed by the subjects, whereas, in the case of estimating the degradation of cartilages, the network tries to segment different tissues and bones of the knee. 

To determine the impairment of individual subjects within the impaired population, we calculate the FID distance between their feature representations and the healthy population's feature representations. If a subject's feature representations are similar to those of the healthy population, their FID distance will be relatively low, suggesting that they are less impaired. Conversely, if a subject's feature representations are significantly different from those of the healthy population, their FID distance will be higher, suggesting that they are more impaired.
